# Supplementary material for: Correlated and anti-correlated density dependent motility
Source: arXiv:2602.01414 source file (2026-02-01)
Supplement: Supplementary file 1 [file Supplemental_Material.pdf]

# Correlated and anti-correlated density dependent motility

Itay Azizi

## Supplemental Material

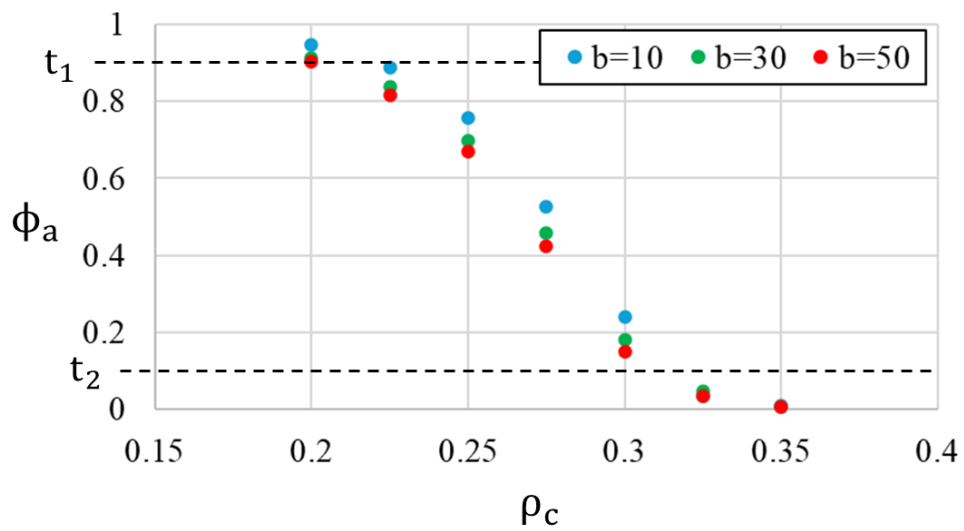

Fig.S1 Correlated case: active fraction as a function of critical density.

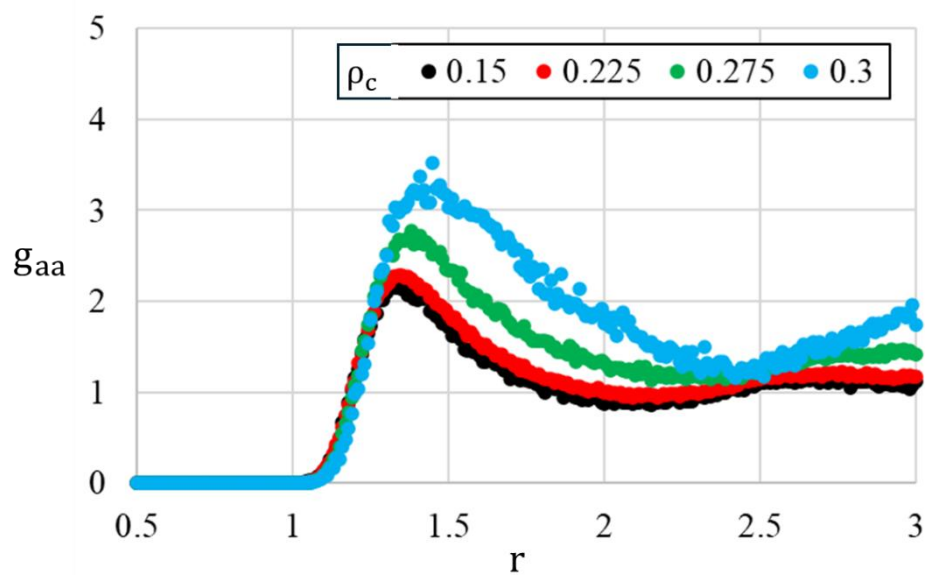

Fig.S2 Correlated case: active radial distribution functions at  $b = 30$ .

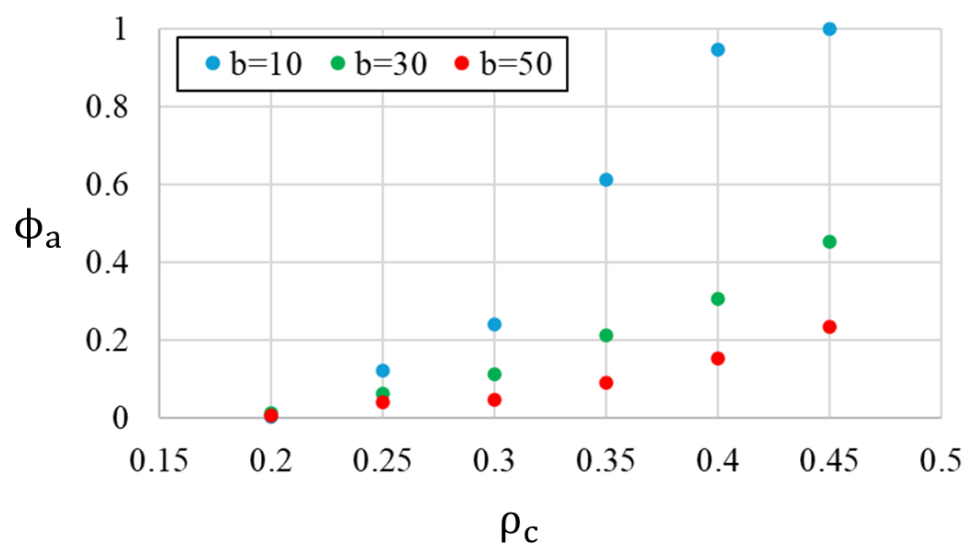

Fig.S3 Anti-correlated case: active fraction as a function of critical density.

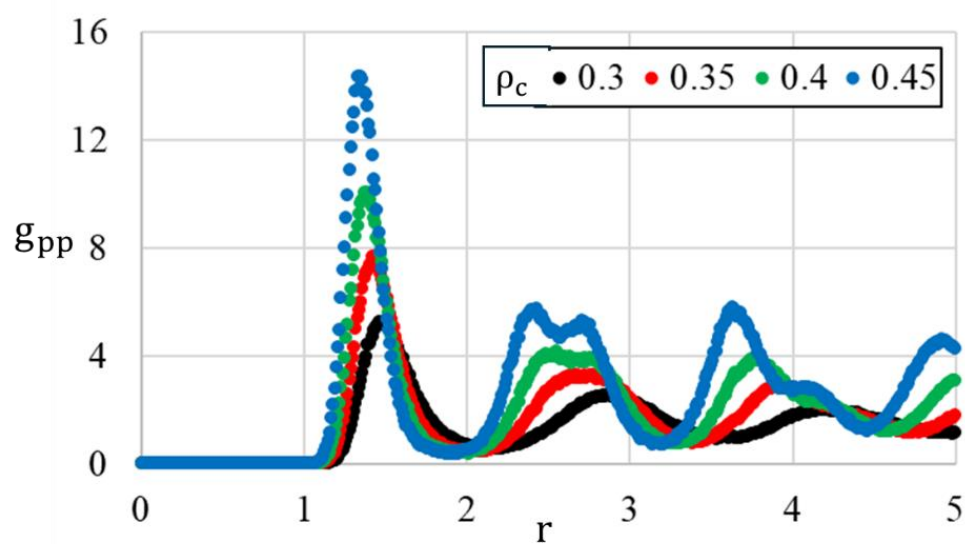

Fig.S4 Anti-correlated case: passive radial distribution functions at  $b = 30$ .
